# Supplementary material for: Deep-MPC: A DAGGER-Driven Imitation Learning Strategy for Optimal Constrained Battery Charging
Source: arXiv:2406.15985 source file (2024-06-23)
Supplement: Supplementary file 1 [file appendix_battery_model.tex]

\textcolor{red}{The primary categories of models used in sophisticated battery management systems (BMSs) include equivalent circuit models (ECMs) \cite{he2011evaluation, nejad2016systematic} and electrochemical models (EMs) \cite{gomadam2002mathematical, ramadesigan2012modeling}. ECMs are relatively simple and intuitive, whereas EMs offer a comprehensive explanation of the electrochemical processes occurring within a cell. Electrochemical models are more appropriate for simulation purposes rather than for real-time control applications. Furthermore, the implementation of electrochemical models in a control framework is constrained by issues of identifiability and observability \cite{moura2015estimation}. As a result, researchers have been focusing on the creation of simplified electrochemical models that are quicker to simulate, identifiable, observable, and still provide adequate representation of the internal cell phenomena \cite{zou2014control, zou2015framework}. The single-particle model (SPM) \cite{Santhanagopalan2006}, which is obtained from the pseudo-two-dimensional model \cite{Doyle1993} by considering the two electrodes as spherical particles, is one notable example among these models. SPM is used in this paper to mathematically describe the battery dynamics. Such a simplified electrochemical model has been largely adopted for battery control and estimation of the states, due to its ability in achieving a reasonable trade-off between the computational cost and accuracy (see \mbox{\eg \cite{Pozzi2020_ifac, pozzi2022lexicographic, Perez2016_spm_1_temperature, Pozzi2022_ccta}).} The accuracy of such a model was demonstrated in \cite{Moura2017}, among others. Note that the battery model is enriched with the two-state temperature dynamics proposed by the authors in \cite{Perez2017a_spme_2_temperature} to account for thermal phenomena.}

\textcolor{red}{Only the equations pertaining to the primary variables of the model are mentioned below; for a more comprehensive explanation, the reader is directed to reference \cite{Pozzi2022_ccta}. Specifically, the variable $\text{soc}(t) \in [0,\,1]$ represents the state of charge of the battery, whose temporal evolution is given by:
\begin{align}\label{eq:soc}
\frac{d\,\text{soc}(t)}{d\,t} = \frac{I(t)}{3600 C}
\end{align}
where the applied current is denoted as $I(t)$, with the convention that a positive current charges the cell and $C$ represents the cell capacity in $[\text{Ah}]$. 
 It is important to note that when the battery is fully charged, the state of charge is at $\text{soc}(t)=1$, and when completely discharged, the state of charge is at $\text{soc}(t)=0$. Moreover, the battery voltage is given by the following equation:
\begin{align}\label{eq:voltage}
V(t) = U_p(t)-U_n(t)+\eta_p(t)-\eta_n(t)+R_{sei}I(t)
\end{align}
where the terms $U_i(t)$ and $\eta_i(t)$, for $i\in\{n,p\}$, represent the open circuit potential and overpotential, respectively, as defined in Section 2 of \cite{Pozzi2022_ccta}, while the term $R_{sei}I(t)$ describes the voltage drop in the solid electrolyte interphase (SEI) resistance. Note that the open circuit potentials and the overpotential are nonlinear functions of the applied current, state of charge, and battery average temperature. As far as the latter is concerned, the two-state model proposed in \cite{Perez2017a_spme_2_temperature} is adopted here for the thermal dynamics, in which the core and the surface temperatures are represented by $T_c(t)$ and $T_s(t)$, respectively. In particular, it holds that:
\begin{subequations}\label{eq:temperature_dynamics}
\begin{align}
C_c\frac{d\,T_c(t)}{d\,t}=& \,Q(t)-\frac{T_c(t)-T_s(t)}{R_{c,s}}\\
C_s\frac{d\,T_s(t)}{d\,t} =& \, \frac{T_c(t)-T_s(t)}{R_{c,s}}-\frac{T_s(t)-T_{env}}{R_{s,e}}
\end{align}
\end{subequations}
where $R_{c,s}$ and $R_{s,e}$ denote the thermal resistances between the core and surface and between the surface and the external environment, respectively, whereas $C_c$ and $C_s$ represent, respectively, the heat capacity of the cell's core and surface. Finally, $Q(t)$ represents the amount of heat generated, which is defined as follows:
\begin{align}\label{eq:heat_generation}
Q(t)=& |I(t)(V(t)- U_p(t)+U_n(t))|.
\end{align}}

 \textcolor{red}{It is important to highlight that the electrochemical parameters in nominal form have been extracted from the experimental characterization of a commercial cell, specifically the Kokam SLPB 75106100, as presented in \cite{Ecker2015, Ecker2015a}, while the thermal ones are based on those employed by \cite{Perez2017a_spme_2_temperature}.}
